# Supplementary material for: A Universal Framework for Compressing Embeddings in CTR Prediction
Source: arXiv:2502.15355 source file (2025-02-21)
Supplement: Supplementary file 1 [file 7_appendix.tex]

\section{Analysis of Hyper-Parameter.}
\label{app:hyper}

    As shown in Figure \ref{fig:line_chart}, we conducted a comprehensive analysis of crucial hyper-parameters in our proposed MEC framework, specifically focusing on the regularization loss coefficient ($\alpha$), contrastive loss coefficient ($\beta$), embedding dimension after quantization ($d$), and number of embedding layers following quantization ($m$).

    For the coefficients $\alpha$ and $\beta$, we systematically tested a range of values, specifically $[0.1, 0.01, 0.001, 0.0001]$, and determined that $\alpha = 0.001$ and $\beta = 0.01$ produced the best performance. 
    Adjusting these values either too high or too low disrupted the optimization balance, leading to underfitting or overfitting.  
    
    The embedding dimension $d$ was assessed using values from a parameter list as $[256, 512, 1024, 2048]$. We found that an embedding dimension of $2048$ yielded the optimal performance. 
    Smaller dimensions resulted in excessive information loss during quantization, which made feature modeling overly coarse. 
    However, as the embedding dimension increased, the performance improvements began to diminish due to the formation of numerous empty cluster centers, which did not significantly enhance the model.  
    
    Finally, we examined the number of embedding layers $m$ using values of $[2, 4, 8]$. 
    We discovered that utilizing $4$ embedding layers led to the best performance. A smaller value of $m$ resulted in inadequate richness in the quantized embeddings, affecting modeling quality, while a larger $m$ caused the segmented vectors to contain insufficient information, hindering the modeling of relationships among different dimensions of the embedding vectors.

\section{\textbf{Analysis of Pre-train Models}}
\label{app:pretrain_models}
    To evaluate the impact of various pre-trained models on our framework, we conducted experiments employing FM \cite{FM}, DeepFM \cite{DeepFM}, and DCNv2 \cite{DCNv2} as the pre-training models for embedding generation and subsequent quantization. In the context of downstream CTR prediction tasks, we used PNN \cite{PNN} to assess the performance of the quantized embeddings within a recommendation system.
    
    The experimental results, presented in Table \ref{tab:pretrain_model_analysis}, demonstrate that while there are minor variations in downstream task performance when utilizing embeddings from different pre-trained models, these differences are negligible. This finding indicates that our framework exhibits robust generalizability across a range of pre-trained models.
    
    This characteristic is particularly beneficial in industrial applications, as it enables the use of smaller, less complex models to generate embeddings without significantly compromising performance. Consequently, our framework facilitates efficient and effective deployment across various practical scenarios.

\section{\textbf{Analysis of Pre-train Models}}

We evaluated the impact of different pre-trained models (FM \cite{FM}, DeepFM \cite{DeepFM}, DCNv2 \cite{DCNv2}) on our framework for embedding generation and quantization, using PNN for downstream CTR prediction. Table \ref{tab:pretrain_model_analysis} shows minor performance variations across models, highlighting our framework's robust generalizability. This enables the use of simpler models in industrial applications without significant performance loss, allowing efficient deployment in various scenarios.

\section{Visualization Analysis}
\label{app:visual}

    To illustrate the effectiveness of MEC, we conducted a case study utilizing a two-dimensional visualization of selected codes from the Criteo dataset based on the PNN \cite{PNN} model. Specifically, we aimed to demonstrate the impact of incorporating popularity-weighted regularization and contrastive learning during quantization, comparing results with and without these methods. We focused on the "C16" feature from the Criteo dataset, selecting the 400 codes with the highest number of assigned features for visualization. In this representation, each cell indicates the number of features assigned to each code, with darker colors signifying higher frequencies.  
    \begin{figure}[ht]
        \centering
        \includegraphics[width=\textwidth]{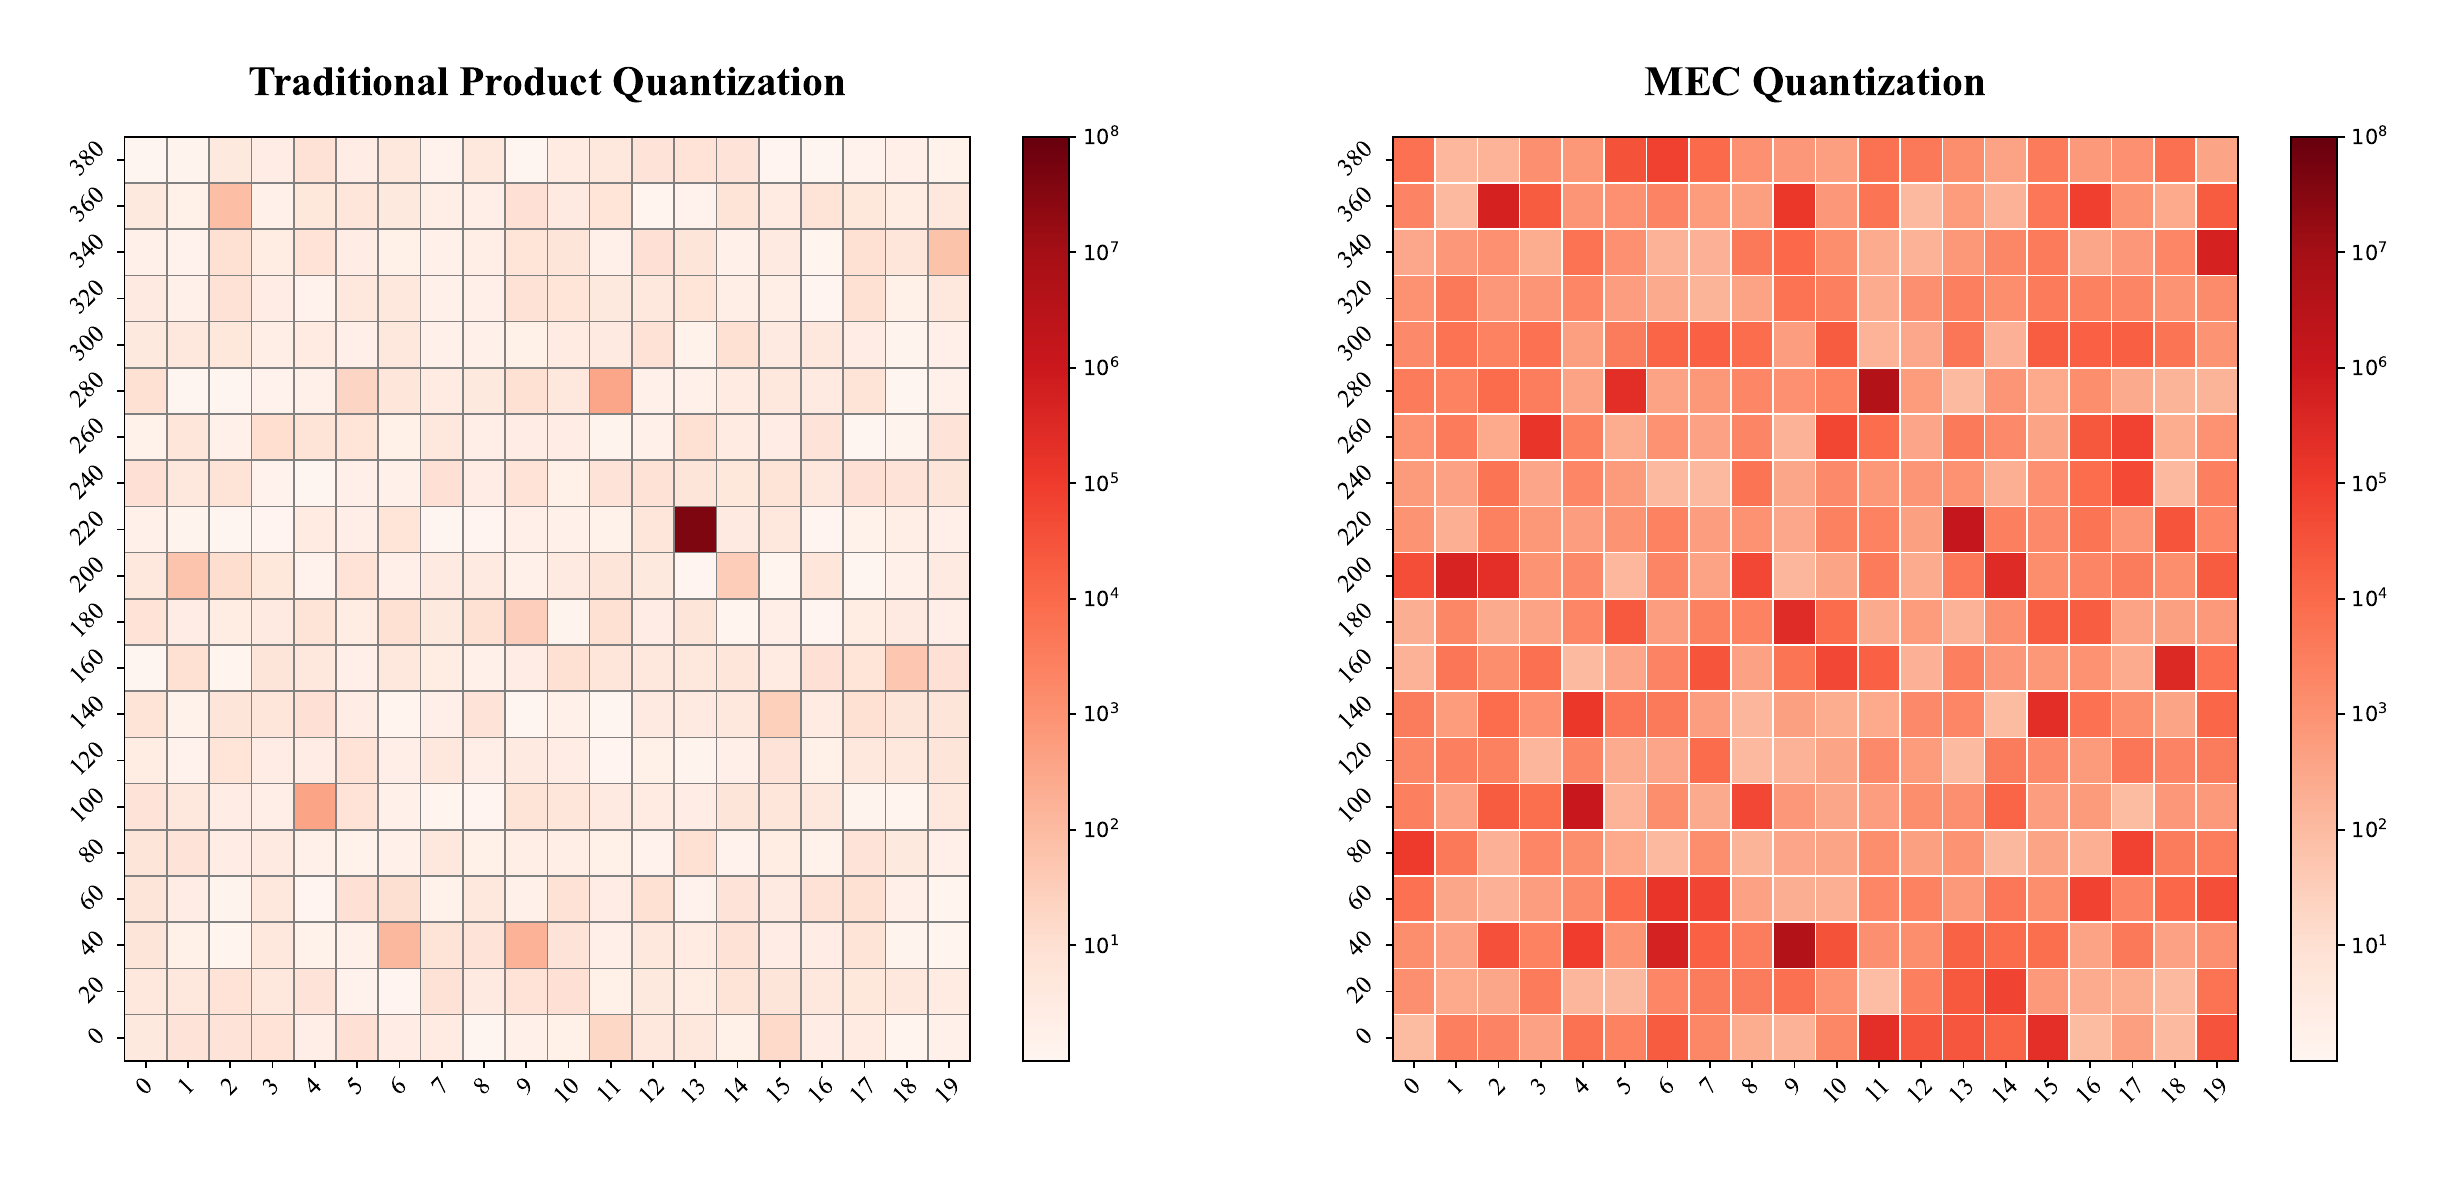}
        \caption{Code Distributions Visualization}
    \label{fig:heatmap}
    \vspace{-10pt}
    \end{figure}
    The left side of the figure displays results obtained using a conventional frequency-only PQ method. This distribution is markedly uneven, with a few cells exhibiting very dark colors and almost all the cells appearing very light. This indicates that clustering embeddings solely based on frequency leads to highly skewed results, resulting in suboptimal code distribution quality. In contrast, the right side of the figure presents the outcomes obtained through MEC. After the application of regularization and contrastive learning, the distribution becomes significantly more uniform.  
    
    This outcome demonstrates that our model effectively balances feature frequencies across codes, culminating in a more equitable and high-quality code distribution. The visualization underscores the advantages of MEC in generating balanced and effective embeddings compared to traditional PQ methods. By integrating regularization and contrastive learning, MEC addresses the issues associated with imbalanced clustering and enhances the overall quality of the embedding space.

\section{Analysis of Training Latency}
\label{app:latency}
In this section, we analyze the training latency, given the computational constraints in real-world scenarios where training time needs careful consideration. 
To compare the time consumption of different modules in the improved training process, we analyzed the latency during the pre-training stage with various quantization methods: (1) w/o PQ indicates no quantization is used, involving only the auxiliary CTR model training time; (2) origin PQ applies the original PQ quantization method; (3) w/o cons. uses PQ quantization with popularity regularization weighting; (4) w/o reg applies PQ quantization with contrastive learning; (5) $\text{MEC}_{PNN}$ employs the complete pre-training method.

Results are shown in Table \ref{tab:Latency}, based on the Criteo and Avazu datasets, with each experiment averaged over 10 repetitions. 
From the results, it is evident that the training time required for the PQ component is negligible compared to the auxiliary CTR model's training latency. 
Additionally, the popularity-weighted regularization does not increase time complexity. 
Although adding contrastive learning slightly increases the time, it remains acceptable relative to the overall training duration.
This demonstrates the practicality of our approach, significantly enhancing the quality of quantized embeddings without noticeably increasing training latency.

Table \ref{tab:Latency} presents the results based on the Criteo and Avazu datasets, averaged over 10 runs. The PQ component adds negligible training time compared to the main CTR model. Popularity-weighted regularization does not increase time complexity, and while contrastive learning slightly increases training time, it remains manageable. Overall, our approach improves quantized embedding quality without significantly impacting training latency.
